# Supplementary material for: Adversarial Learning of General Transformations for Data Augmentation
Source: arXiv:1909.09801 source file (2019-09-21)
Supplement: Supplementary file 1 [file additional_material.tex]

\documentclass[10pt,twocolumn,letterpaper]{article}

\usepackage{iccv}
\usepackage{times}
\usepackage{epsfig}
\usepackage{graphicx}
\usepackage{amsmath}
\usepackage{amssymb}
\usepackage{algorithm}
\usepackage{algorithmic}
\usepackage{caption}
\usepackage{subcaption}
\usepackage{pgfplots}
\usepackage{comment}
\usepackage{tikz}
\usetikzlibrary{tikzmark}

\usepackage{tabulary,multirow}

\newcolumntype{x}[1]{>{\centering\arraybackslash}p{#1pt}}

\newlength\savewidth

\makeatletter\renewcommand\paragraph{\@startsection{paragraph}{4}{\z@}
  {.5em \@plus1ex \@minus.2ex}{-.5em}{\normalfont\normalsize\bfseries}}\makeatother

\usepackage{array}
\newcolumntype{L}[1]{>{\raggedright\let\newline\\\arraybackslash\hspace{0pt}}m{#1}}
\newcolumntype{C}[1]{>{\centering\let\newline\\\arraybackslash\hspace{0pt}}m{#1}}
\newcolumntype{R}[1]{>{\raggedleft\let\newline\\\arraybackslash\hspace{0pt}}m{#1}}

% Include other packages here, before hyperref.

% If you comment hyperref and then uncomment it, you should delete
% egpaper.aux before re-running latex.  (Or just hit 'q' on the first latex
% run, let it finish, and you should be clear).
\usepackage[pagebackref=true,breaklinks=true,colorlinks,bookmarks=false]{hyperref}

%\iccvfinalcopy % *** Uncomment this line for the final submission

 % *** Enter the ICCV Paper ID here

% Pages are numbered in submission mode, and unnumbered in camera-ready
\ificcvfinal\pagestyle{empty}\fi

\begin{document}

%%%%%%%%%%%%%%%%%%%%%%
% TITLE
%%%%%%%%%%%%%%%%%%%%%%
\title{Adversarial Learning of General Transformations for Data Augmentation\\ Supplementary Material}

%%%%%%%%%%%%%%%%%%%%%%
% AUTHORS
%%%%%%%%%%%%%%%%%%%%%%
\author{Saypraseuth Mounsaveng\\
Ecole de Techonolgie Supérieure\\
Montreal, Canada\\
{\tt\small saypraseuth.mounsaveng.1@etsmtl.net}
\and
Marco Pedersoli\\
Ecole de Techonolgie Supérieure\\
Montreal, Canada\\
{\tt\small marco.pedersoli@etsmtl.ca}
\and
Ismail Ben Ayed\\
Ecole de Techonolgie Supérieure\\
Montreal, Canada\\
{\tt\small ismail.benayed@etsmtl.ca}
\and
David Vazquez\\
Element AI\\
Montreal, Canada\\
{\tt\small dvazquez@elementai.com}
}

\maketitle
%\thispagestyle{empty}

%%%%%%%%%%%%%%%%%%%%%%
% Additional material
%%%%%%%%%%%%%%%%%%%%%%
\section{Training algorithm}
\label{ssec:training}
Our model is trained according to algorithm~\ref{alg:training_algorithm}.
To train our model, we sample different data batches. $batch_i$ is a batch of real samples to be transformed by $G$, $batch_j$ is a batch of real samples used to train $D^C$ and $C$, $batch_k$ is a batch of real samples with the same labels as in $batch_i$ and used to train $D^D$  and finally $batch_z$ is a batch of noise samples used by $G$ in combination with $batch_i$ to create new samples.\\
During training, all elements of the model are updated in a sequential order, first the two discriminators $D^C$ and $D^D$, then the generator $G$ and finally the classifier $C$.

\begin{algorithm}
\caption{Minibatch stochastic gradient descent training of our model - Fully supervised}
\label{alg:training_algorithm}
\begin{algorithmic}[1]
    \FOR{nIter}
            \STATE Sample $batch_i$ of $m$ labeled pairs $(x_i,y_i)\sim~p_{data}$ 
            \STATE Sample $batch_j$ of $m$ labeled pairs $(x_j,y_j)\sim~p_{data}$ 
            \STATE Sample $batch_z$ of $m$ of noise samples $z \sim p_z$ 
            %\STATE Compute $\mathcal{L}_{D^C}$ 
            \STATE Update $D^C$ by:\\ % descending its stochastic gradient:
            $\begin{aligned}
                \nabla_{\theta_{D^C}} &\frac{1}{m}\sum_{n=1}^{m}[\log{(D^C(x_j^{(n)}, y_j^{(n)}))}\\
                &+ \log{(1 - D^C(G(x_i^{(n)}, z^{(n)}), y_i^{(n)}))}]
            \end{aligned}$
            \STATE Sample batch of $m$ pairs $(x_k,y_k) \sim p_{data}$  with same labels as $batch_i$
            %\STATE Compute $\mathcal{L}_{D^{D}}$
            \STATE Update $D^D$ by:\\ %descending its stochastic gradient:
            $\begin{aligned}
               \nabla_{\theta_{D^D}} &\frac{1}{m}\sum_{n=1}^{m} [\log{(D^D(x_i^{(n)}, x_k^{(n)}))} \\
                &+ \log{(1-D^D(x_i, G(x_i^{(n)}, z^{(n)})))}]
            \end{aligned}$
            %\STATE Compute $\mathcal{L}_{G}$
            \STATE Update $G$ by:\\ %descending its stochastic gradient:
            $\begin{aligned}
                \nabla_{\theta_{G}} &\frac{1}{m}\sum_{n=1}^{m} [\alpha\log{(D^C_{y_i}(G(x_i^{(n)}, z^{(n)}), y_i^{(n)}))} \\ 
                &+ \beta\log{(D^D(x_i, G(x_i^{(n)}, z^{(n)})))}] \\
                &+ \gamma\log{(1-C_{y_i}(G(x_i^{(n)}))}]
            \end{aligned}$
            %\STATE Compute $\mathcal{L}_{C}$
            \STATE Update $C$ by:\\ % descending its stochastic gradient:
            $\begin{aligned}
                \nabla_{\theta_{C}} &\frac{1}{m}\sum_{n=1}^{m} [\log{(C_{y_j}(x_j^{(n)}))} \\
                &+  \log{(C_{y_i}(G(x_i^{(n)},z^{(n)})))}]
            \end{aligned}$
    \ENDFOR
\end{algorithmic}
\end{algorithm}

\section{Hyper-parameters}
All hyper-parameters are selected based on the performance on a validation set.
For all the sub-networks we used Adam as optimizer with a learning rate of 0.0005. Just for the classifier $C$ we noticed that its learning rate is important to obtain the best performance. In this case we use a learning rate of 0.001, 0.0005, 0.006, 0.0001 for MNIST, SVHN, CIFAR10 and FMNIST respectively.
In Tab.~\ref{tab:hyperparameters} we report the optimal hyper-parameters associated to the importance of each term in the generator loss $\mathcal{L}_G$
Tab.~\ref{tab:hyperparameters} shows the training hyper parameter values. 
%To chose those values, an hyper parameter search was done by training the model with the training dataset and measuring its performance on a validation set.
\begin{table}[ht]
\renewcommand\thetable{4}
\centering
\footnotesize
\begin{tabular}{c|c|c|c|c}
Balance factors for $\mathcal{L}_G$ & MNIST & SVHN & CIFAR10 & FMNIST \\
\hline
% Learning rate & & &\\
% $D^D$ & 0.0005 & 0.0005 & 0.0005 & 0.0005\\
% $D^C$ & 0.0005 & 0.0005 & 0.0005 & 0.0005\\
% $G$ & 0.0005 & 0.0005 & 0.0005 & 0.0005\\
% $C$ & 0.001 & 0.0005 & 0.006 & 0.0001\\
%Learning rate $C$ & 0.001 & 0.0005 & 0.006 & 0.0001\\
%Balance factors for $\mathcal{L}_G$ & & &\\%\multicolumn{4}{c}{\dotfill} \\
$\alpha$ & 0.1 & 1 & 0.1 & 0.1\\ 
$\beta$ & 0.05 & 1 & 0.05 & 0.05\\
$\gamma$ & 0.005 & 0.0005 & 0.001 & 0.005\\
\end{tabular}
%}
\caption{\textbf{Training hyper parameters for each dataset}. }
\label{tab:hyperparameters}
\end{table}

\section{Detailed architectures}
In this section, we detail the networks used for all experiments. In Tab.~\ref{tab:DC}, Tab.~\ref{tab:DD}, Tab.~\ref{tab:G} and Tab.~\ref{tab:C} we report the architecture of respectively the two discriminators $D^C$ and $D^D$, the generator $G$ and the classifier $C$.
The architecture of $D^C$, $D^D$ and $C$ is adapted from the discriminator architecture of [7]. The only difference is that the first layer of $D^C$ and $D^D$ was adapted to handle respectively the class information and an additional image as additional input and the last layer of $C$ was adapted to perform multi class classification.
All models expect input images of size 32x32, which correspond to the image size of CIFAR10 and SVHN dataset. In order to use MNIST and FMNIST images that are of size 28x28 with our networks, we zero pad them with two pixels. Images can be color (3 input channels, for SVHN and CIFAR10) or grayscale (1 input channel for FMNIST and MNIST).

\begin{table}[H]
\renewcommand\thetable{5}
\centering
\footnotesize
%\resizebox{\columnwidth}{!}{%
\begin{tabular}{p{3.8cm}|c}
\multicolumn{2}{c}{\textbf{Discriminator $D^C$}}\\
\hline
Input 32x32 image & Input one-hot class representation\\
% \hline
3x3 conv. 48 LReLU(0.2) & 32x32 deconv. 48 LReLU(0.2)\\
% merge
\multicolumn{2}{c}{concat}\\
\multicolumn{2}{c}{3x3 conv. 96 LReLU(0.2),weight norm}\\
\multicolumn{2}{c}{3x3 conv. 96 LReLU(0.2),weight norm}\\
\multicolumn{2}{c}{0.5 dropout} \\
\multicolumn{2}{c}{3x3 conv. 192 LReLU(0.2),weight norm}\\
\multicolumn{2}{c}{3x3 conv. 192 LReLU(0.2),weight norm}\\
\multicolumn{2}{c}{3x3 conv. 192 LReLU(0.2),weight norm}\\
\multicolumn{2}{c}{0.5 dropout}\\
\multicolumn{2}{c}{3x3 conv. 192 LReLU(0.2),weight norm}\\
\multicolumn{2}{c}{1x1 conv. 192 LReLU(0.2),weight norm}\\
\multicolumn{2}{c}{1x1 conv. 192 LReLU(0.2),weight norm}\\
\multicolumn{2}{c}{MLP 1 unit, sigmoid}
\end{tabular}
%}
\caption{\textbf{Architecture of $D^C$}. The class discrimnator takes as input a 32x32 image and the one-hot representation of its class label. Both inputs are transformed into an equal number of feature maps of same size and then concatenated to form an input for the rest of the network.}
\label{tab:DC}
\end{table}

\begin{table}[H]
\renewcommand\thetable{6}
\centering
\footnotesize
%\resizebox{\columnwidth}{!}{%
\begin{tabular}{c|c}
\multicolumn{2}{c}{\textbf{Discriminator $D^D$}}\\
\hline
Input 32x32 image & Input 32x32 image\\
%\hline
3x3 conv. \tikzmark{e}48 LReLU(0.2) & 3x3 conv. 48\tikzmark{f} LReLU(0.2) \\
\multicolumn{2}{c}{\tikzmark{g}concat\tikzmark{h}}\\
\multicolumn{2}{c}{3x3 conv. 96 LReLU(0.2),weight norm}\\
\multicolumn{2}{c}{3x3 conv. 96 LReLU(0.2),weight norm}\\
\multicolumn{2}{c}{0.5 dropout}\\
\multicolumn{2}{c}{3x3 conv. 192 LReLU(0.2),weight norm}\\
\multicolumn{2}{c}{3x3 conv. 192 LReLU(0.2),weight norm}\\
\multicolumn{2}{c}{3x3 conv. 192 LReLU(0.2),weight norm}\\
\multicolumn{2}{c}{0.5 dropout}\\
\multicolumn{2}{c}{3x3 conv. 192 LReLU(0.2),weight norm}\\
\multicolumn{2}{c}{1x1 conv. 192 LReLU(0.2),weight norm}\\
\multicolumn{2}{c}{1x1 conv. 192 LReLU(0.2),weight norm}\\
\multicolumn{2}{c}{MLP 1 unit, sigmoid}
\end{tabular}
%}
\caption{\textbf{Architecture of $D^D$}. The dissimilarity discriminator takes as input two 32x32 images. Both images are transformed into an equal number of feature maps of same size and then concatenated to form an input for the rest of the network.}
\label{tab:DD}
\end{table}

\begin{table}[H]
\renewcommand\thetable{7}
\centering
\footnotesize
\begin{tabular}{c|c}
\multicolumn{2}{c}{\textbf{Generator G}}\\
\hline
\multicolumn{2}{c}{\textit{\dotfill~Part 1: UNET down branch, $E_{NC}$ in equ. 1~\dotfill}}\\
Input 32x32 image & Input 100-dim noise vector\\
3x3 conv. 32,batchNorm,LReLU(0.2) & -\\
3x3 conv. 32,batchNorm,LReLU(0.2) & 32x32 deconv. 32, LReLU(0.2)\\
\multicolumn{2}{c}{concat}\\
\multicolumn{2}{c}{2x2 max-pooling}\\
\multicolumn{2}{c}{3x3 conv. 64,batchNorm,LReLU(0.2)}\\
\multicolumn{2}{c}{3x3 conv. 128,batchNorm,LReLU(0.2)}\\
\multicolumn{2}{c}{2x2 max-pooling}\\
\multicolumn{2}{c}{3x3 conv. 256,batchNorm,LReLU(0.2)}\\
\multicolumn{2}{c}{3x3 conv. 256,batchNorm,LReLU(0.2)}\\
\multicolumn{2}{c}{2x2 max-pooling}\\
\multicolumn{2}{c}{3x3 conv. 512,batchNorm,LReLU(0.2)}\\
\multicolumn{2}{c}{3x3 conv. 512,batchNorm,LReLU(0.2)}\\
\multicolumn{2}{c}{2x2 max-pooling}\\
\multicolumn{2}{c}{3x3 conv. 1024,batchNorm,LReLU(0.2)}\\
\multicolumn{2}{c}{3x3 conv. 1024,batchNorm,LReLU(0.2)}\\
% \multicolumn{2}{c}{\textit{\dotfill~STN, $T$ in equ. 1~\dotfill}}\\
% \multicolumn{2}{c}{MLP 32 unit, ReLU}\\
% \multicolumn{2}{c}{MLP 6 unit}\\
% \multicolumn{2}{c}{\textit{\dotfill~Part 2: UNET down branch, $E_{NC}$ in equ. 1~\dotfill}}\\
% Transformed 32x32 image & input 100-dim noise vector\\
% 3x3 conv. 32,batchNorm,LReLU(0.2) & -\\
% 3x3 conv. 32,batchNorm,LReLU(0.2) & 32x32 deconv. 32, LReLU(0.2)\\
% \multicolumn{2}{c}{2x2 max-pooling}\\
% \multicolumn{2}{c}{3x3 conv. 64,batchNorm,LReLU(0.2)}\\
% \multicolumn{2}{c}{3x3 conv. 128,batchNorm,LReLU(0.2)}\\
% \multicolumn{2}{c}{2x2 max-pooling}\\
% \multicolumn{2}{c}{3x3 conv. 256,batchNorm,LReLU(0.2)}\\
% \multicolumn{2}{c}{3x3 conv. 256,batchNorm,LReLU(0.2)}\\
% \multicolumn{2}{c}{2x2 max-pooling}\\
% \multicolumn{2}{c}{3x3 conv. 512,batchNorm,LReLU(0.2)}\\
% \multicolumn{2}{c}{3x3 conv. 512,batchNorm,LReLU(0.2)}\\
% \multicolumn{2}{c}{2x2 max-pooling}\\
% \multicolumn{2}{c}{3x3 conv. 1024,batchNorm,LReLU(0.2)}\\
% \multicolumn{2}{c}{3x3 conv. 1024,batchNorm,LReLU(0.2)}\\
\multicolumn{2}{c}{\textit{\dotfill~Part 2: UNET up branch, $D_{EC}$ in equ. 1~\dotfill}}\\
\multicolumn{2}{c}{3x3 conv. 512,batchNorm,LReLU(0.2)}\\
\multicolumn{2}{c}{3x3 conv. 512,batchNorm,LReLU(0.2)}\\
\multicolumn{2}{c}{3x3 conv. 256,batchNorm,LReLU(0.2)}\\
\multicolumn{2}{c}{3x3 conv. 256,batchNorm,LReLU(0.2)}\\
\multicolumn{2}{c}{3x3 conv. 128,batchNorm,LReLU(0.2)}\\
\multicolumn{2}{c}{3x3 conv. 128,batchNorm,LReLU(0.2)}\\
\multicolumn{2}{c}{3x3 conv. 64,batchNorm,LReLU(0.2)}\\
\multicolumn{2}{c}{3x3 conv. 64,batchNorm,LReLU(0.2)} \\
\multicolumn{2}{c}{1x1 conv. 3 for color, 1 for grayscale}\\
\end{tabular}
%}
\caption{\textbf{Architecture of G}. The Generator takes as input a 32x32 image and a 100 dimensional noise vector and processes them in 2 steps. In a first step, $G$ encodes the input image and a noise vector into a feature vector using $E_{NC}$. This is passed to a 2-layer MLP outputing the parameters of an affine transformation $T$, as in Equ.(1). In a second step, this learned transformation is applied to the original input image, which is concatenated with same 100 dimensional noise vector and given to UNET. UNET, which is the composition of $E_{NC}$ and $D_{EC}$, will generate the final image. For a better understanding see Fig.(1) of the main paper. }
\label{tab:G}
\end{table}

\begin{table}[H]
\renewcommand\thetable{8}
\centering
\footnotesize
\begin{tabular}{c}
\textbf{Classifier C}\\
\hline
Input 32x32 tmage\\
\hline
3x3 conv. 96 LReLU(0.2),weight norm\\
3x3 conv. 96 LReLU(0.2),weight norm\\
3x3 conv. 96 LReLU(0.2),weight norm\\
0.5 dropout\\
3x3 conv. 192 LReLU(0.2),weight norm\\
3x3 conv. 192 LReLU(0.2),weight norm\\
3x3 conv. 192 LReLU(0.2),weight norm\\
0.5 dropout\\
3x3 conv. 192 LReLU(0.2),weight norm\\
3x3 conv. 192 LReLU(0.2),weight norm\\
3x3 conv. 192 LReLU(0.2),weight norm\\
MLP 10 unit, sigmoid\\
10-class Softmax\\
\end{tabular}
%}
\caption{\textbf{Architecture of $C$}. $C$ is a standard classifier composed of multiple convolutional layers. It takes as input a 32x32 image and outputs the probability that it belongs to each defined class.}
\label{tab:C}
\end{table}

%\subsection{Additional image examples}

\end{document}
